# Supplementary material for: Support Size Estimation: The Power of Conditioning
Source: arXiv:2211.11967 source file (2022-11-22)
Supplement: Supplementary file 1 [file appendix.tex]

\section{Proof of Lemma~\ref{upperboundonI}} 
\label{app:upperboundonI}
 We have 
 \[
I = \int_{z_i} \sum_{s\in S^c} g_s p_s(z_i) \log \frac{  p_s(z_i)}{\sum_{s \in S^c}g_s p_s(z_i)} \,dz_i
\]
\[
 =  \sum_{s\in S^c} \int_{z_i}  g_s p_s(z_i) \log \frac{  p_s(z_i)}{\sum_{s \in S^c}g_s p_s(z_i)} \,dz_i
\]
\[
 = \sum_{s\in l_0} \int_{z_i}   g_s p_s(z_i) \log \frac{  p_s(z_i)}{\sum_{s \in S^c}g_s p_s(z_i)} \,dz_i + \sum_{s\in l_1} \int_{z_i}   g_s p_s(z_i) \log \frac{  p_s(z_i)}{\sum_{s \in S^c}g_s p_s(z_i)} \,dz_i +\sum_{s\in l_d} \int_{z_i}   g_s p_s(z_i) \log \frac{  p_s(z_i)}{\sum_{s \in S^c}g_s p_s(z_i)} \,dz_i 
 \]
 \[
+  \sum_{s\in \Bar{S}} \int_{z_i}   g_s p_s(z_i) \log \frac{  p_s(z_i)}{\sum_{s \in S^c}g_s p_s(z_i)} \,dz_i
\]
Recall that  $p_s(0) = 1$ (and $p_s(z_i) = 0$ for $z_i \neq 0$)  when $s \in L_0$, $p_s(1) = 1$ when $s \in L_1$ and $p_s(z^*) = 1$ for some $z^*$ (recall that $z^* = \sum_{j \in [i-1]}\beta_j z_j$)  when $s \in L_d$. Also note that $0 \log 0 = 0$. So we have 
\[
\sum_{s\in L_0} \int_{z_i}   g_s p_s(z_i) \log \frac{  p_s(z_i)}{\sum_{s \in S^c}g_s p_s(z_i)} \,dz_i = \sum_{s\in L_0} g_s \log \frac{1}{\sum_{s \in S^c}g_s p_s(0)}
\]
Note that $p_s(0) = 0$ for $s \not \in L_0$ and hence
\[
\sum_{s\in L_0} \int_{z_i}   g_s p_s(z_i) \log \frac{  p_s(z_i)}{\sum_{s \in S^c}g_s p_s(z_i)} \,dz_i = \sum_{s\in L_0} g_s \log \frac{1}{\sum_{s \in L_0}g_s} = (\sum_{s\in L_0} g_s) \frac{1}{\sum_{s \in L_0}g_s}
\]

Similarly, we have 
\[
\sum_{s\in L_1} \int_{z_i}   g_s p_s(z_i) \log \frac{  p_s(z_i)}{\sum_{s \in S^c}g_s p_s(z_i)} \,dz_i =  (\sum_{s\in L_1} g_s) \frac{1}{\sum_{s \in L_1}g_s}
\]

Note that for $s \in \Bar{S}$, even though $z_i$ can take a fixed value $z^*$ but $p_s(z^*) = 0$ as $p_s(\cdot)$ is a continuous distribution a shown before. This will imply, similar to previous cases: 

\[
\sum_{s\in L_d} \int_{z_i}   g_s p_s(z_i) \log \frac{  p_s(z_i)}{\sum_{s \in S^c}g_s p_s(z_i)} \,dz_i =  (\sum_{s\in L_d} g_s) \frac{1}{\sum_{s \in L_d}g_s}
\]

Note that $(\sum_{s\in L_0} g_s) \frac{1}{\sum_{s \in L_0}g_s}+(\sum_{s\in L_1} g_s) \frac{1}{\sum_{s \in L_1}g_s}+(\sum_{s\in L_d} g_s) \frac{1}{\sum_{s \in L_d}g_s} \le \log 3$. Now we upper bound $
\sum_{s\in \Bar{S}} \int_{z_i}   g_s p_s(z_i) \log \frac{  p_s(z_i)}{\sum_{s \in S^c}g_s p_s(z_i)} \,dz_i$. Since $p_s(\cdot)$ is a continuous distribution (so $p_s(z^*) = 0$ for any fixed $z^*$) so $\sum_{s\in \Bar{S}} \int_{z_i}   g_s p_s(z_i) \log \frac{  p_s(z_i)}{\sum_{s \in S^c}g_s p_s(z_i)} \,dz_i = \sum_{s\in \Bar{S}} \int_{z_i}   g_s p_s(z_i) \log \frac{  p_s(z_i)}{\sum_{s \in \Bar{S}}g_s p_s(z_i)} \,dz_i$

Now,
\[
\sum_{s\in \Bar{S}} \int_{z_i}   g_s p_s(z_i) \log \frac{  p_s(z_i)}{\sum_{s \in \Bar{S}}g_s p_s(z_i)} \,dz_i = \sum_{s\in \Bar{S}} g_s \int_{z_i}    p_s(z_i) \log \frac{  p_s(z_i)}{\sum_{s \in \Bar{S}}g_s p_s(z_i)} \,dz_i
\]

\[
= \sum_{s\in \Bar{S}} g_s KL(p_s(z_i)||\Bar{p}(z_i))%\int_{z_i}    p_s(z_i) \log \frac{  p_s(z_i)}{\sum_{s \in \Bar{S}}g_s p_s(z_i)} \,dz_i
\]

where $\Bar{p}(z_i)= \sum_{s \in \Bar{S}}g_s p_s(z_i)$. From the convexity of KL divergence, we have $KL(p_s(z_i)||\Bar{p}(z_i)) \le \sum_{s' \in \Bar{S}}g_{s'}KL(p_s,p_{s'})$. Therefore, $\sum_{s\in \Bar{S}} g_s KL(p_s(z_i)||\Bar{p}(z_i)) \le \sum_{s,s' \in \Bar{S}}g_s g_{s'} KL(p_s(z_i),p_{s'}(z_i)) \le (\sum_{s \in \Bar{S}} g_s)^2 \max_{s,s' \in \Bar{S}}KL(p_s(z_i),p_{s'}(z_i)) = \max_{s,s' \in \Bar{S}} KL(p_s(z_i),p_{s'}(z_i)) =O(1)$ (the last  equality is due to Lemma \ref{lem:bouldedkl}). Finally, $I \le \log 3 + O(1) = O(1)$.

\iffalse

\paragraph*{Remaining Proof of Theorem \ref{thm:upperbound}}
If $t^* = 0$ then the algorithm returns $|\mathcal{S}|$ exactly. So assume $t^* \ge 1$. Let $\Bar{t}$ be the value of $t$ such that $12/\epsilon^2 \le |\mathcal{S}|/2^{\Bar{t}}  < 24/\epsilon^2$. Now,
\begin{align*}
&\Pr[|2^{t^*} X_{t^*} - |\mathcal{S}|| > \epsilon |\mathcal{S}|] \\
&= Pr[ |X_{t^*} - |\mathcal{S}|/2^{t^*}| > \epsilon |\mathcal{S}|/2^{t^*}]\\
&= Pr[ |X_{t^*} - E[X_{t^*}]| > \epsilon E[X_{t^*}]]\\
&= \sum_{i =1}^{\log n} Pr[ |X_{t} - E[X_{t}]| > \epsilon E[X_{t}]|t = t^*] Pr[t = t^*]\\
&= \sum_{i =1}^{\Bar{t}-1} Pr[ |X_{t} - E[X_{t}]| > \epsilon E[X_{t}]|t = t^*] Pr[t = t^*] +\sum_{\Bar{t}}^{\log n} Pr[ |X_{t} - E[X_{t}]| > \epsilon E[X_{t}]|t = t^*] Pr[t = t^*]\\
&\le \sum_{i =1}^{\Bar{t}-1} Pr[ |X_{t} - E[X_{t}]| > \epsilon E[X_{t}]] + \sum_{\Bar{t}}^{\log n} Pr[t = t^*]\\
&=  \sum_{i =1}^{\Bar{t}-1} Pr[ |X_{t} - E[X_{t}]| > \epsilon E[X_{t}]] + \sum_{\Bar{t}}^{\log n} Pr[X_{t-1} > c/\epsilon^2, X_t \le c/\epsilon^2]\\
&\le \sum_{i = 1}^{\Bar{t}-1}\frac{Var[X_t]}{\epsilon^2 E^2[X_t]}+ Pr[X_{\Bar{t}-1} > c/\epsilon^2]\\
&\le  \sum_{i = 1}^{\Bar{t}-1}\frac{1}{\epsilon^2 E[X_t]}+ E[X_{\Bar{t}-1}] \epsilon^2/c\\
&= \sum_{i =1}^{\Bar{t}-1}\frac{2^t}{\epsilon^2 |\mathcal{S}|} + \frac{|\mathcal{S}|\epsilon^2}{c 2^{\Bar{t}-1}} = \frac{2^t}{\epsilon^2 |\mathcal{S}|}+\frac{|\mathcal{S}|}{2^{\Bar{t}}} \frac{2\epsilon^2}{c} = 1/6
\end{align*}
\qed

\fi
